# Supplementary material for: Indium as a high cooling power nuclear refrigerant for quantum nanoelectronics
Source: arXiv:1811.03034 ancillary file (2020-03-04)
Supplement: Supplementary file 1 [file supplement.pdf]

# Supplementary Information

# Indium as a high cooling power nuclear refrigerant for quantum nanoelectronics

Nikolai Yurttagül,[1,*] Matthew Sarsby,[1,*] and Attila Geresdi[1,†]

[1] *QuTech and Kavli Institute of Nanoscience, Delft University of Technology, 2600 GA Delft, The Netherlands*

[*] These authors contributed equally to this work.

[†] Corresponding author; e-mail: a.geresdi@tudelft.nl

## DEVICE FABRICATION

The bottom electrode was deposited by DC magnetron sputtering (AJA ATC 1800-V, base pressure $8.7 \cdot 10^{-10}$ mbar, 4 inch substrate holder) of 180 nm Al (2 inch target, 99.9995% Al, Kurt J. Lesker) onto a Si/$SiO_2$ wafer, with 0.19 W/cm$^2$ (DC-power 60 W, DC bias 336 V) at 4.7 µbar Ar pressure. The substrate to target distance was 10 cm (tilted 45°) with 20 rpm substrate rotation. Right after unloading the sample, 2.2 µm AZ-nLOF 2020 (Microchemicals GmbH) is spincoated (4000 rpm, softbake 110 °C on a hotplate) and patterned using electron beam lithography (RAITH Voyager, 50 kV acceleration voltage, 60 µm aperture, 2.1 nA beam current, dose 44 µC/µm$^2$). The resist is developed in AZ-726 MIF (Microchemicals GmbH) after a crosslinking bake at 110 °C on a hotplate. The Al bottom electrode is then patterned by wet etching using a commercial etching mixture (Al etchantType D, Transene). The resist was removed by Technistrip NI555 (Microchemicals GmbH) at 60°C.

The 230 nm $SiO_2$ thick interlayer dielectric was deposited by RF-sputtering using an Alliance AC450 system with a base pressure $1.1{\cdot}10^{-7}$ mbar and 4 inch substrate holder (4 inch target, 99.99% $SiO_2$) yielding 0.39 W/cm$^2$ (RF-power 125 W, DC-Bias 141 V) at 8 µbar Ar pressure. The substrate to target distance was 8 cm (no tilt) without substrate rotation. The vias are defined by spin coating 130 nm AR-P 6200.13 (Allresist GmbH, 4000 rpm, softbake at 150 °C on a hotplate) and patterned by electron beam lithography (RAITH Voyager, 50 kV acceleration voltage, 30 µm aperture, 0.1 nA beam current, dose 218 µC/µm$^2$). The resist is developed in AR-600-546 (Allresist GmbH). Vias trough the $SiO_2$ interlayer dielectric are then etched by RIE (Oxford PlasmaPro 100 Estrelas) using 0.66 W/cm$^2$ (RF-power 120 W, DC bias -270 V) in pure $CHF_3$ (50 sccm) at a pressure of 6.7 µbar and 15° C with 13 mbar He backing. The resist is removed in AR 300-76 at room temperature.

To define the tunnel junctions, the chip was loaded into the AJA ATC 1800-V and the bottom Al electrode was depassivated by ion milling (15 min in 0.31 W/cm$^2$ RF-plasma (RF-power 100 W, -286 V DC-bias) at 4 µbar Ar pressure). The device was transferred in Ar flow into the loadlock (base pressure $< 1{\cdot}10^{-7}$ mbar) where tunnel barriers were formed by oxidation in 99.999% pure $O_2$ at a pressure of 105 mbar and room temperature for 140 min. The chip was then loaded into the main chamber in vacuo followed by in-situ DC magnetron

sputtering of 260 nm Al as top electrode. The deposition and patterning of the top electrode was performed in the same way as for the bottom electrode.

The device was capped by RF-magnetron sputtering (Alliance AC450) of 70 nm $SiO_2$ with 0.39 W/$cm^2$ (RF-power 125 W, DC-Bias 141 V) at 8 µbar Ar pressure. The substrate to target distance was 8 cm (no tilt) without substrate rotation. 2.7 µm AZ ECI 3027 (Microchemicals GmbH) was spin coated (4000 rpm, softbake 100 °C, hotplate) followed by patterning with laser lithography (MicroWriter ML2, Durham Magneto Optics Ltd, 405 nm exposure wavelength, dose 210 mJ/$cm^2$) and RIE (Oxford ICP100, process gases $SF_6$, $Cl_2$, $CHF_3$, HBr) using 0.15 W/$cm^2$ (RF-power 50 W, DC bias -235 V) in pure $SF_6$ (30 sccm) at a pressure of 8 µbar and room temperature with 13 mbar He backing. The Si carrier wafer was coated with 500 nm Cr in order to increase the DC bias. The resist is removed in AZ 100 (Microchemicals GmbH). To avoid loss of material due to ion milling of the top electrode the lithography and etching process is performed alternating on the top electrode (etch depth 70 nm $SiO_2$) and bottom electrode (etch depth 300 nm $SiO_2$).

The exposed Al was depassivated by ion-beam milling (250 eV ion energy, 80 nA ion current in 0.7 µbar Ar pressure) and the seed layer of 270 nm Cu (0.5 nm/s, 20° tilt) and 30 nm Au (0.1 nm/s) was deposited by electron beam evaporation (Alliance EVA 450, base pressure $8.3 \cdot 10^{-8}$ mbar, 7.4 kV emission voltage) on a water cooled substrate holder. As masking layer for the electrodeposition process, 35 µm AZ 40XT (Microchemicals GmbH) was spin coated (2000 rpm, soft-bake ramp from 60 °C to 125 °C). The mask was patterned by laser lithography (1 µm resolution, 375 nm exposure wavelength, dose 800 mJ/$cm^2$) and developed in AZ 726 MIF (Microchemicals) after a post exposure bake (ramp from 60 °C to 105 °C). Prior to electroplating, the seed layer was cleaned by 30 s immersion in 2.5% TMAH (aq) and 1 min $O_2$ plasma clean (200 W, 200 sccm $O_2$ without substrate bias) to avoid skip plating. The electroplating process was performed at room temperature in a stirred aqueous solution of 0.26 M $In(SO_3NH_2)_3$ (Indium Corporation) using 99.99% pure In as the counterelectrode. The galvanostatic process is performed (PGSTAT 204, Metrohm) in a three-electrode setup using a AgCl/Cl reference electrode (regenerated in 4M KCl) to measure the electrochemical potential. The cell current duty cycle was 1.5 ms 16 mA/$cm^2$ (0.39 V, forward), 0.5 ms -16 mA/$cm^2$ (-0.39 V, reverse) and 8 ms 0 mA giving rise to a net deposition rate of 0.04 nm per cycle. A 110 min electroplating process thus resulted in a 25.4 µm thick coating, smooth enough to follow the patterning resolution of the mask. The

mask is removed in DMSO at room temperature followed by the removal of the seed layer in $I_2$/KI (10 g KI and 2.5 g $I_2$ in 100 ml DI $H_2O$).

## ADDITIONAL DATASETS

The single island capacitance was extracted at low temperatures by fitting the full single electron tunneling model to the voltage-dependent conductance, $G(V)$. Comparing devices with different geometries (Fig. S1) establishes that the island capacitance $C_\Sigma$ scales linearly with the island overlap area, $A_L = 2w_L \times d_L$. The intersect of 77 fF at zero $A_L$ defines the sum of the stray capacitance of the island, $C_0$ and the capacitance of the two tunnel junctions.

| Device | $N$ | $w_L \times d_L$ (µm×µm) | $C_\Sigma$ (fF) | island area (µm×µm) | In block $w \times d \times t$(µm×µm×µm) |
|---|---|---|---|---|---|
| 1 | 36 | $100 \times 18$ | $479 \pm 2$ | $100 \times 120$ | $140 \times 50 \times 25.4$ |
| 2 | 36 | $160 \times 18$ | $673 \pm 8$ | $120 \times 160$ | $140 \times 50 \times 25.4$ |
| 3 | 26 | $400 \times 14$ | $1285 \pm 10$ | $250 \times 400$ | $420 \times 160 \times 25.4$ |

TABLE S1. **Geometry and island capacitance of three devices.** The dimensions are defined in Fig. 1 of the main text. We discuss device 1 in the main text.

The deviation at $|V/N| > 7.5\,\mu$V from theory towards smaller $G/G_t$ can be explained with overheating and scales as expected with the island area in the way that only device 1 is affected by it. Devices 2 and 3 show good agreement between the single electron tunneling model and measured charging curves over the whole bias range.

We characterize the junction resistivity and its standard deviation at room temperature by fabricating an array where each individual junction is accessible in a four-wire measurement geometry. We find a resistivity and standard deviation of $12.8 \pm 0.8\,\mathrm{k\Omega \mu m^2}$.

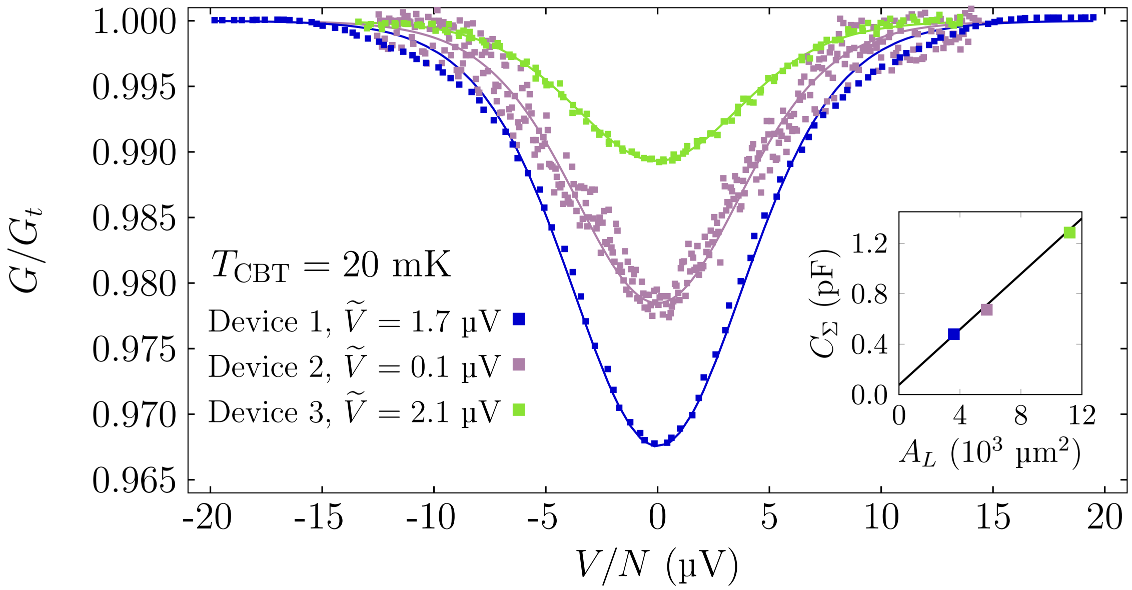


FIG. S1. **Comparison of the three CBT devices listed in Table S1.** Note that the voltage bias, V is scaled with the array length, $N$. All measurements were taken at $T_{\mathrm{CBT}} = 20\,\mathrm{mK}$ and at $B = 40\ldots50\,\mathrm{mT}$. The legend shows the device designation (see Table S1 for device layout) and the peak-to-peak voltage excitation amplitude per junction. The inset shows the extracted $C_\Sigma$ as a function of the overlap area, $A_L = 2w_L \times d_L$ between adjacent islands.

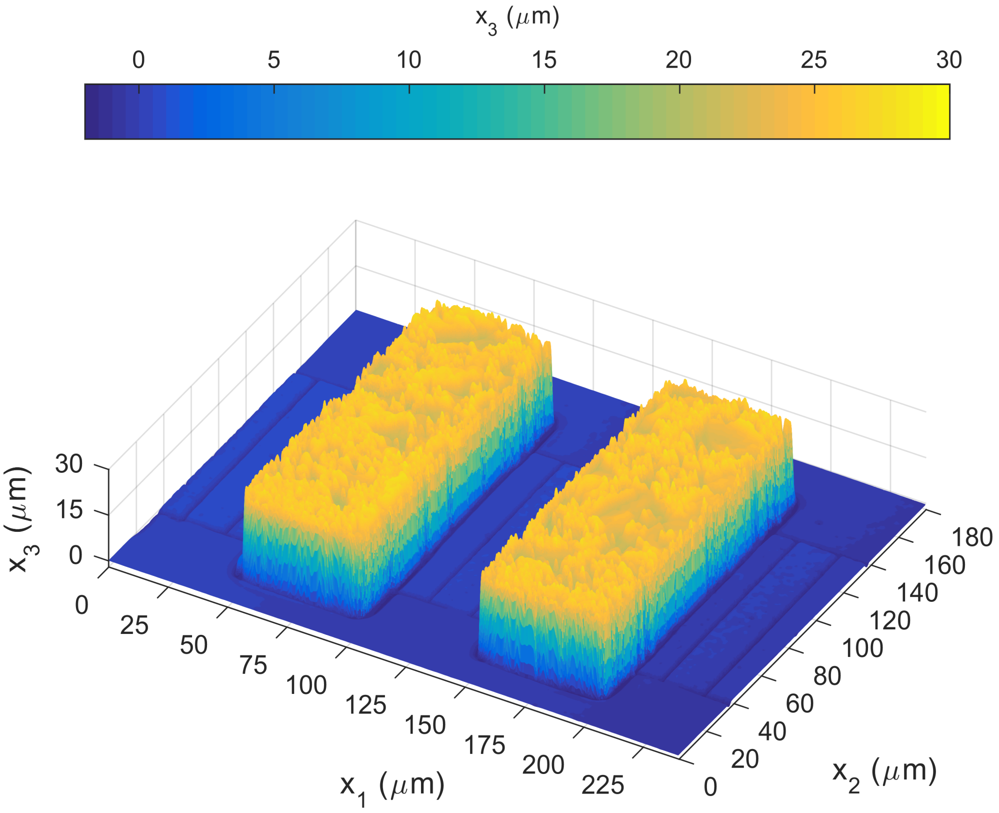


FIG. S2. **Height profile of the indium cooling fins.** The height map was created by a white light interference microscope with a horizontal step size of 240 nm.
